# Supplementary material for: Read Pointer Meters in complex environments based on a Human-like Alignment and Recognition Algorithm
Source: arXiv:2302.14323 source file (2023-07-30)
Supplement: Supplementary file 1 [file appendix.tex]

\section{Digital meter recognition}
\label{appendix}
While this article focuses on reading pointer meters, we demonstrate in Fig.\ref{figdigital} how to easily read digital meters using off-the-shelf optical character recognition (OCR) models. To be more precise, we consider the digital meter recognition task to be a standard scene text spotting problem and thus construct an independent model with the same architecture as the meter numbering recognition branch in Sec \ref{sec:method}. We can achieve reasonable results in digital meter recognition by detecting and recognizing the bounding boxes.
\\
Future work could focus on developing a unified model capable of simultaneously recognizing pointers and digital meters.
